# Supplementary material for: Transactions on Red-black and AVL trees in NVRAM
Source: arXiv:2006.16284 source file (2020-06-29)
Supplement: Supplementary file 1 [file avl-insert-sm.tex]

\begin{tikzpicture}
  \begin{scope}[>=stealth,x=2.5mm,y=2.5mm]
  \clip (-1.6,17.7) rectangle (13.6,37.3);
  %%\sffamily%%
  \smaller\smaller\smaller
  \let\sizebox\relax
  \newlength{\sizebox}\setlength{\sizebox}{2.8mm}

  \tikzstyle{box}=[draw,circle,inner sep=0pt,align=center,text width=1.5\sizebox,minimum size=1.8\sizebox,text height=1.5ex,text depth=.25ex]

  %% states
  \node[box,double] (clean) at (5,37) {C};
  \node[box,fill=gray!30!white] (A1) at (0,35.6) {A1};
  \node[box,fill=gray!30!white] (A2) at (3.5,33.6) {A2};
  %%\node[box,fill=gray!30!white] (A3) at (9,31) {A3};
  \node[box,fill=gray!30!white] (A4) at (3.5,30.4) {A4};
  %%\node[box,fill=gray!30!white] (A5) at (2,31) {A5};
  %%\node[box,fill=gray!30!white] (A6) at (2,24) {A6};
  \node[box,fill=gray!30!white] (A7) at (0,26.2) {A7};
  \node[box,fill=gray!30!white] (A8) at (0,23) {A8};
  \node[box,fill=gray!30!white] (A9) at (4,19.8) {A9};
  \node[box,fill=gray!30!white] (A10) at (4,26.2) {A10};
  \node[box,fill=gray!30!white] (A11) at (0,19.8) {A11};
  \node[box,fill=gray!30!white] (A12) at (4,23) {A12};
  \node[box,fill=gray!30!white] (A13) at (8,23) {A13};
  \node[box,fill=gray!30!white] (A14) at (8,26.2) {A14};

  \node[box,fill=gray!30!white] (A15) at (8.5,29.4) {A15};
  \node[box,fill=gray!30!white] (A16) at (8,19.8) {A16};
  \node[box,fill=gray!30!white] (A17) at (12,19.8) {A17};
  \node[box,fill=gray!30!white] (A18) at (12,23) {A18};
  \node[box,fill=gray!30!white] (A19) at (12,26.2) {A19};
  \node[box,fill=gray!30!white] (A20) at (12,29.4) {A20};

  \node[box,fill=gray!30!white] (A21) at (12,32.6)  {A21};
  \node[box,fill=gray!30!white] (A22) at (6.5,33.6)  {A22};
  \node[box,fill=gray!30!white] (A23) at (11,35.6) {A23};
  \node[box,fill=gray!30!white] (A24) at (8,37) {A24};

  \node[box,fill=gray!30!white] (A25) at (0,32.6) {A25};
  \node[box,fill=gray!30!white] (A26) at (0,29.4) {A26};

  %% transitions
  \sffamily%%

  \draw[dashed,->] (clean) to[bend left=10] (A1);
  \draw[->] (clean) -- (A2);

  \draw[->] (A1) to[bend left=10] node[sloped,pos=0.5,above=2pt] {new}  (clean); % insert new node

  \draw[dashed,->] (A2) -- (A25); %% init variables

  \draw[->] (A4) to[out=60,in=-90] (clean);  % insert new node
  \draw[->] (A4) -- (A7); % insert new node

  \draw[dashed,->] (A7) -- (A8);
  \draw[dashed,->] (A7) -- (A10);

  \draw[dashed,->] (A8) -- (A11);

  \draw[dashed,->] (A9) -- (A12);

  \draw[dashed,->] (A10) -- (A13);
  \draw[dashed,->] (A10) -- (A22);
  \draw[dashed,->] (A10) to[out=45,in=-120] (A23);

  \draw[->] (A11) -- (A9);

  \draw[dashed,->] (A12) -- (A8);
  \draw[dashed,->] (A12) -- (A10);

  \draw[dashed,->] (A13) -- (A14);
  \draw[dashed,->] (A13) -- (A16);

  \draw[->] (A14) -- (A15);

  \draw[->] (A15) -- (A22) node[sloped,pos=0.6,above=1pt] {rot}; %% rotation
  \draw[->] (A15) -- (A23) node[sloped,pos=0.3,below=1pt] {rot};

  \draw[dashed,->] (A16) -- (A17);

  \draw[->] (A17) -- (A18);

  \draw[dashed,->] (A18) -- (A19);

  \draw[->] (A19) -- (A20) node[sloped,pos=0.4,above=1pt] {rot}; %% rotation

  \draw[dashed,->] (A20) -- (A21);

  \draw[->] (A21) -- (A22) node[sloped,pos=0.7,above=1pt] {rot}; %% rotation
  \draw[->] (A21) -- (A23) node[sloped,pos=0.5,above=3pt] {rot}; %% rotation

  \draw[dashed,->] (A22) -- (clean);

  \draw[dashed,->] (A23) -- (A24);

  \draw[->] (A24) -- (clean);

  \draw[dashed, ->] (A25) -- (A26);

  \draw[dashed,->] (A26) -- (A4);

  \end{scope}
\end{tikzpicture}
