# Supplementary material for: Transactions on Red-black and AVL trees in NVRAM
Source: arXiv:2006.16284 source file (2020-06-29)
Supplement: Supplementary file 2 [file avl-remove-sm.tex]

\begin{tikzpicture}
  \begin{scope}[>=stealth,x=2.5mm,y=2.5mm]
  \clip (-1.6,18.0) rectangle (18.5,37.9);
  %%\sffamily%%
  \smaller\smaller\smaller
  \let\sizebox\relax
  \newlength{\sizebox}\setlength{\sizebox}{2.8mm}

  \tikzstyle{box}=[draw,circle,inner sep=0pt,align=center,text width=1.5\sizebox,minimum size=1.8\sizebox,text height=1.5ex,text depth=.25ex]

  \node[box,double] (clean) at (7.0,30) {C};
  \node[box,fill=gray!30!white] (R1) at (3.5,36.4) {R1};
  \node[box,fill=gray!30!white] (R2) at (0.0,36.4) {R2};
  \node[box,fill=gray!30!white] (R3) at (3.5,33.2) {R3};
  \node[box,fill=gray!30!white] (R4) at (1.8,28.6) {R4};
  \node[box,fill=gray!30!white] (R5) at (4.5,30.1) {R5};
  \node[box,fill=gray!30!white] (R6) at (3.7,26.2) {R6};
  \node[box,fill=gray!30!white] (R7) at (0,33.2) {R7};
  \node[box,fill=gray!30!white] (R8) at (0,30) {R8};
  \node[box,fill=gray!30!white] (R9) at (0,26.8) {R9};
  \node[box,fill=gray!30!white] (R10) at (0,23.6) {R10};
  \node[box,fill=gray!30!white] (R11) at (0,20.4) {R11};
  \node[box,fill=gray!30!white] (R12) at (3.5,20.4) {R12};
  \node[box,fill=gray!30!white] (R13) at (3.5,23.6) {R13};
  \node[box,fill=gray!30!white] (R14) at (7,23.6) {R14};

  \node[box,fill=gray!30!white] (R15) at (10.5,30) {R15};
  \node[box,fill=gray!30!white] (R16) at (10.5,26.8) {R16};
  \node[box,fill=gray!30!white] (R17) at (7,20.4) {R17};
  \node[box,fill=gray!30!white] (R18) at (10.5,20.4) {R18};
  \node[box,fill=gray!30!white] (R19) at (14,20.4) {R19};
  \node[box,fill=gray!30!white] (R20) at (7.0,26.8) {R20};

  \node[box,fill=gray!30!white] (R21) at (10.5,23.6)  {R21};
  \node[box,fill=gray!30!white] (R22) at (16.2,25.3)  {R22};
  \node[box,fill=gray!30!white] (R23) at (14,30) {R23};
  \node[box,fill=gray!30!white] (R24) at (14,36.4) {R24};

  \node[box,fill=gray!30!white] (R25) at (10.5,36.4) {R25};
  \node[box,fill=gray!30!white] (R26) at (7.0,36.4) {R26};

  \node[box,fill=gray!30!white] (R27) at (10.5,33.2) {R27};
  \node[box,fill=gray!30!white] (R28) at (14,23.6) {R28};
  \node[box,fill=gray!30!white] (R29) at (14,26.8) {R29};
  \node[box,fill=gray!30!white] (R30) at (17.2,20.4) {R30};
  \node[box,fill=gray!30!white] (R31) at (14,33.2) {R31};
  \node[box,fill=gray!30!white] (R32) at (17.2,30) {R32};
  \node[box,fill=gray!30!white] (R33) at (17.2,33.2) {R33};
  \node[box,fill=gray!30!white] (R34) at (17.2,36.4) {R34};

  %% transitions
  \sffamily%%

  \draw[dashed,->] (clean) to[bend right=7] (R1);
  \draw[dashed,->] (clean) to[out=40,in=90,looseness=2.7] (clean);

  \draw[->] (R1) to[bend right=7] (clean);
  \draw[->] (R1) -- (R2);
  \draw[->] (R1) to[bend right=22] (R4);
  \draw[->] (R1) -- (R7);

  \draw[dashed,->] (R2) to[bend right=10] (R3);

  \draw[->] (R3) -- (clean);
  \draw[->] (R3) to[bend right=10] (R2);
  \draw[->] (R3) -- (R4);
  \draw[->] (R3) -- (R7);

  \draw[dashed,->] (R4) -- (R5);
  \draw[dashed,->] (R4) -- (R6);

  \draw[->] (R5) -- (R20);

  \draw[dashed,->] (R6) -- (R20);

  \draw[->] (R7) -- (R8);

  \draw[->] (R8) -- (R9);
  \draw[->] (R8) to[bend right=28] (R11);

  \draw[dashed,->] (R9) to[bend right=10] (R10);
  \draw[dashed,->] (R9) to[bend left=35] (R11);

  \draw[->] (R10) to[bend right=10] (R9);
  \draw[->] (R10) -- (R11);

  \draw[->] (R11) -- (R12);

  \draw[dashed,->] (R12) -- (R13);

  \draw[->] (R13) -- (R20);

  \draw[dashed,->] (R14) -- (R17);

  \draw[->] (R15) -- (R20);

  \draw[dashed,->] (R16) -- (R20);

  \draw[->] (R17) to[bend right=35] (clean); %%to[out=-30,in=30,looseness=2.6]
  \draw[->] (R17) -- (R18);
  \draw[->] (R17) to[bend left=30] (R20);

  \draw[dashed,->] (R18) -- (R19);
  \draw[dashed,->] (R18) to[bend right=30] (R30);
  \draw[dashed,->] (R18) -- (R21);

  \draw[->] (R19) -- (R22);

  \draw[dashed,->] (R20) -- (R14);
  \draw[dashed,->] (R20) -- (clean);

  \draw[->] (R21) -- (R28);

  \draw[dashed,->] (R22) -- (R23);

  \draw[->] (R23) -- (R15); %% rotation
  \draw[->] (R23) -- (R16);

  \draw[dashed,->] (R24) -- (R25);

  \draw[->] (R25) -- (R26); %% rotation

  \draw[dashed,->] (R26) -- (R27);

  \draw[->] (R27) -- (R15); %% rotation
  \draw[->] (R27) to[bend right=35] (R16);

  \draw[dashed,->] (R28) -- (R29);

  \draw[->] (R29) -- (R15); %% rotation
  \draw[->] (R29) -- (R16);

  \draw[dashed,->] (R30) to[out=82,in=-60,looseness=1.0] (R31);
  \draw[dashed,->] (R30) to[out=82,in=-74,looseness=1.0] (R32);
  \draw[dashed,->] (R30) to[out=82,in=-66,looseness=1.0] (R33);

  \draw[->] (R31) -- (R34);

  \draw[->] (R32) to[bend left=30] (R34);

  \draw[->] (R33) -- (R34);

  \draw[->] (R34) -- (R24);

  \end{scope}
\end{tikzpicture}
